# Supplementary material for: State-Reification Networks: Improving Generalization by Modeling the Distribution of Hidden Representations
Source: arXiv:1905.11382 source file (2019-05-26)
Supplement: Supplementary file 1 [file appendix.tex]

\section{Attractor net details}

The attractor nets we explore are discrete-time nonlinear dynamical systems.
Given a static $n$-dimensional input $\cue$, the network state at iteration
$k$, $\bm{a}_k$, is updated according to:
\begin{equation}
\bm{a}_{k} = f \left( \bm{W} \bm{a}_{k-1} + \cue \right) ,
\label{eq:att_dyn}
\end{equation}
where $f$ is a nonlinearity and $\bm{W}$ is a weight matrix.  Under certain
conditions on $f$ and $\bm{W}$, the state is guaranteed to converge to a
\emph{limit cycle} or \emph{fixed point}. A limit cycle of length $\lambda$
occurs if $\lim_{k\to\infty} \bm{a}_k = \bm{a}_{k+\lambda}$. A fixed point is
the special case of $\lambda=1$.

Attractor nets have a long history starting with the work of
\cite{Hopfield1982} that was partly responsible for the 1980s wave of
excitement in neural networks.  Hopfield defined a mapping from network state,
$\bm{a}$, to scalar \emph{energy} values via an energy (or Lyapunov) function,
and showed that the dynamics of the net perform local energy minimization. The
shape of the energy landscape is determined by weights $\bm{W}$ and input
$\cue$ (Figure~\ref{fig:energy}a).  Hopfield's original work is based on
binary-valued neurons with asynchronous update; since then similar results
have been obtained for certain nets with continuous-valued nonlinear neurons
acting in continuous \citep{Hopfield1984} or discrete time \citep{Koiran1994}.
\begin{figure*}[bt]
   \begin{center}
   \includegraphics[width=4.in]{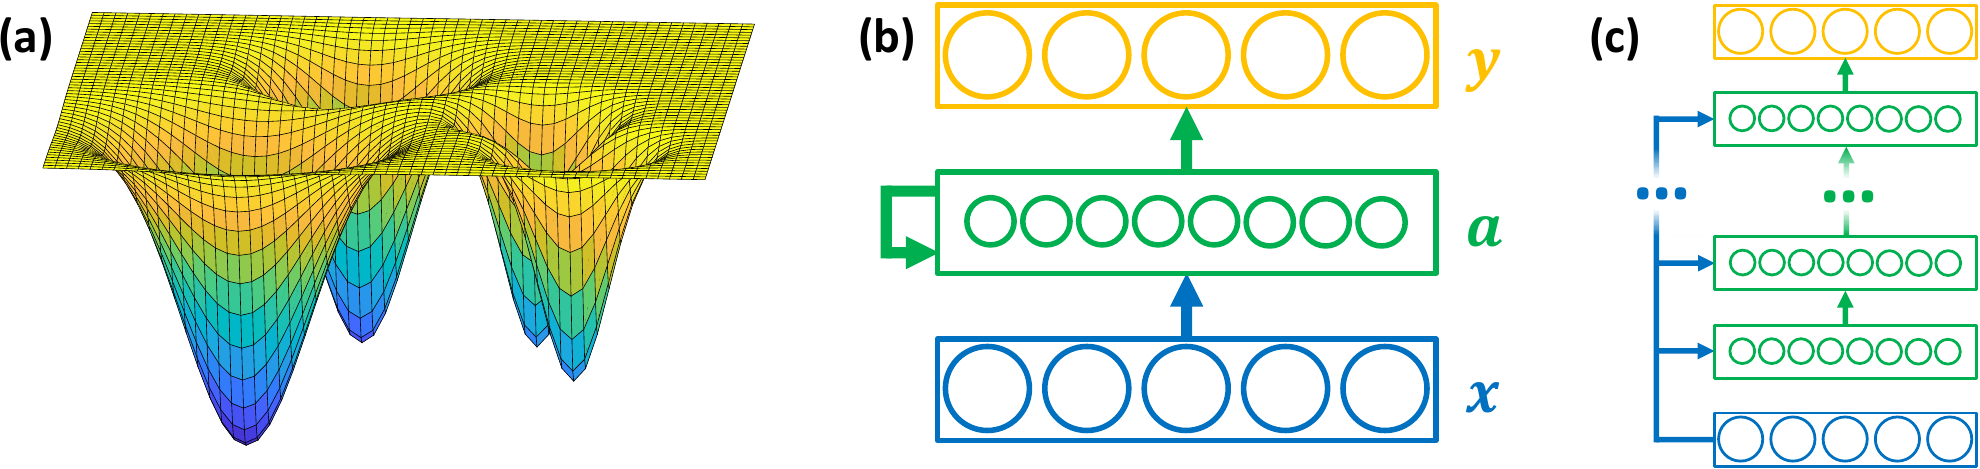}
   \end{center}
   \caption{(a) energy landscape, (b) attractor net, (c) attractor net  unfolded in time.}
   \label{fig:energy}
\end{figure*}
We adopt Koiran's \citeyear{Koiran1994} framework, which dovetails with the
standard deep learning assumption of synchronous updates on continuous-valued
neurons. Koiran shows that with symmetric weights ($w_{ji} = w_{ij}$),
nonnegative self-connections ($w_{ii} \ge 0$), and a bounded nonlinearity $f$
that is continuous and strictly increasing except at the extrema (e.g., tanh,
logistic, or their piece-wise linear approximations), the network asymptotically
converges over iterations to a fixed point or limit cycle of length 2. As a 
shorthand, we refer to convergence in this manner as \emph{stability}.
%In practice, we almost always observe fixed point solutions.

Attractor nets have been used for multiple purposes, including
content-addressable memory, information retrieval, and constraint satisfaction
\citep{Mozer2009,Siegelmann2008}. In each application, the network is 
given an input containing partial or corrupted information, which we will refer
to as the \emph{cue}, denoted $\cue$; and the cue is mapped to
a canonical or \emph{well-formed} output in $\bm{a}_\infty$.
For example, to implement a content-addressable memory, a set of vectors, $\{
\bm{\xi}^{(1)},\bm{\xi}^{(2)},\ldots \}$, must first be stored. The energy landscape is
sculpted to make each $\bm{\xi}^{(i)}$ an attractor via a supervised training
procedure in which the target output is the vector $\bm{\xi}^{(i)}$ for some $i$
and the input $\cue$ is a noise-corrupted version of the target. Following training, noise-corrupted inputs should be `cleaned up' to reconstruct the state.

In the model described by Equation~\ref{eq:att_dyn}, the attractor dynamics operate in the same
representational space as the input (cue) and output. Historically, this is the
common architecture. By projecting the input to a higher dimensional latent
space, we can design attractor nets with greater representational capacity.
Figure~\ref{fig:energy}b shows our architecture, with an
$m$-dimensional input, $\bm{x} \in [-1, +1]^m$, an $m$-dimensional output,
$\bm{y} \in [-1, +1]^m$, and an $n$-dimensional attractor state, $\bm{a}$,
where typically $n > m$ for representational flexibility.  The input $\bm{x}$
is projected to the attractor space via an affine transform:

\begin{equation}
\cue = \Win \bm{x} + \vin .  
\label{eq:cue} 
\end{equation} 
The attractor dynamics operate as in Equation~\ref{eq:att_dyn}, with
initialization $\bm{a}_0 = \bm{0}$ and $f \equiv \mathrm{tanh}$.  Finally, the
asymptotic attractor state is mapped to the output: 
\begin{equation} 
\bm{y} = \fout \left( \Wout \bm{a}_{\infty} + \vout \right) , 
\label{eq:out}
\end{equation} 
where $\fout$ is an output activation function and the $\bm{W}^*$ and
$\bm{v}^*$ are free parameters of the model.

To conceptualize a manner in which this network might operate,  $\Win$ might copy
the $m$ input features forward and the attractor net might use $m$ degrees of
freedom in its state representation to maintain these \emph{visible} features.
The other $n-m$ degrees of freedom could be used as \emph{latent} features that
impose higher-order constraints among the visible features (in much the same
manner as the hidden units in a restricted Boltzmann machine).  When the
attractor state is mapped to the output, $\Wout$ would then transfer only the visible
features.

As Equations~\ref{eq:att_dyn} and \ref{eq:cue} indicate, the input $\bm{x}$
biases the attractor state $\bm{a}_k$ at every iteration $k$, rather than---as
in the standard recurrent net architecture---being treated as an initial value,
e.g., $\bm{a}_0 = \bm{x}$. Effectively, there are short-circuit connections
between input and output to avoid vanishing gradients that arise in deep
networks (Figure~\ref{fig:energy}c). As a result of the connectivity, it is
trivial for the network to copy $\bm{x}$ to $\bm{y}$---and thus to propagate
gradients back from $\bm{y}$ to $\bm{x}$. For example, the network will
implement the mapping $\bm{y} = \bm{x}$ if: $m=n$, $\Win = \Wout  = I$, $\vin =
\vout = \bm{0}$, $\bm{W}=\bm{0}$, and $\fout (\bm{z}) = \bm{z}$ or $\fout (\bm{z}) = \max(-1,\min(+1,\bm{z}))$.
%is the identity mapping or an identity mapping bounded at $-1$ and $+1$.

In our simulations, we use an alternative formulation of the architecture that also enables the copying of $\bm{x}$ to $\bm{y}$ by treating the input as unbounded and imposing a bounding nonlinearity on the output. This variant consists of: the input $\bm{x}$ being replaced with $\hat{\bm{x}} \equiv \mathrm{tanh}^{-1}(\bm{x})$ in Equation~\ref{eq:cue}, $\fout \equiv \mathrm{tanh}$ in Equation~\ref{eq:out}, and the nonlinearity in the attractor dynamics 
being shifted back one iteration, i.e., Equation~\ref{eq:att_dyn} becomes $\bm{a}_{k}
= \bm{W} f(\bm{a}_{k-1}) + \cue$.  This formulation is elegant if $\bm{x}$ is the activation pattern from a layer of tanh neurons, in which case the tanh and $\mathrm{tanh}^{-1}$ nonlinearities cancel. Otherwise, to ensure numerical stability, one can define the input $\hat{\bm{x}} \equiv \mathrm{tanh}^{-1}[(1-\epsilon) \bm{x}]$ for some small 
$\epsilon$.

\subsection{Training a denoising attractor network}
\label{sec:trainingattractor}

We demonstrate the supervised training of a set of attractor states, $\smash{\{\bm{\xi}^{(1)},\bm{\xi}^{(2)},\ldots \bm{\xi}^{(A)}\}}$, 
with ${\smash{\bm{\xi}^{(i)}\sim \mathrm{Uniform}(-1,+1)^m}}$. 
The input to the network is a noisy version of some state $i$, ${\hat{\bm{x}}^{(i)}=\mathrm{tanh}^{-1}(\bm{\xi}^{(i)})+\bm{\eta}}$, 
with $\bm{\eta}\sim \mathcal{N}(\bm{0},\sigma^2 I)$, and the corresponding target output is simply $\bm{\xi}^{(i)}$. With $\kappa$ noisy instances of each attractor for training, we define a normalized denoising loss
\begin{equation}
\mathcal{L}_\mathrm{denoise} = \frac{1}{\kappa A} \sum_{i=1}^{\kappa A} \frac{||\bm{y}^{(i)} - \bm{\xi}^{(i)}||^2}{||\mathrm{tanh}(\hat{\bm{x}}^{(i)}) - \bm{\xi}^{(i)}||^2} ,
\label{eq:denoise}
\end{equation}
to be minimized by stochastic gradient descent. The aim is to sculpt attractor basins whose diameters are related to $\sigma^2$. The normalization in Equation~\ref{eq:denoise} serves to scale the loss such that $\mathcal{L}_\mathrm{denoise} \ge 1$ indicates failure of denoising and $\mathcal{L}_\mathrm{denoise} = 0$ indicates complete denoising. The $[0,1]$ range of this loss helps with calibration when combined with other losses. 

\begin{figure*}[bt]%[100]%[bt]
   \begin{center}
   \includegraphics[width=5.5in]{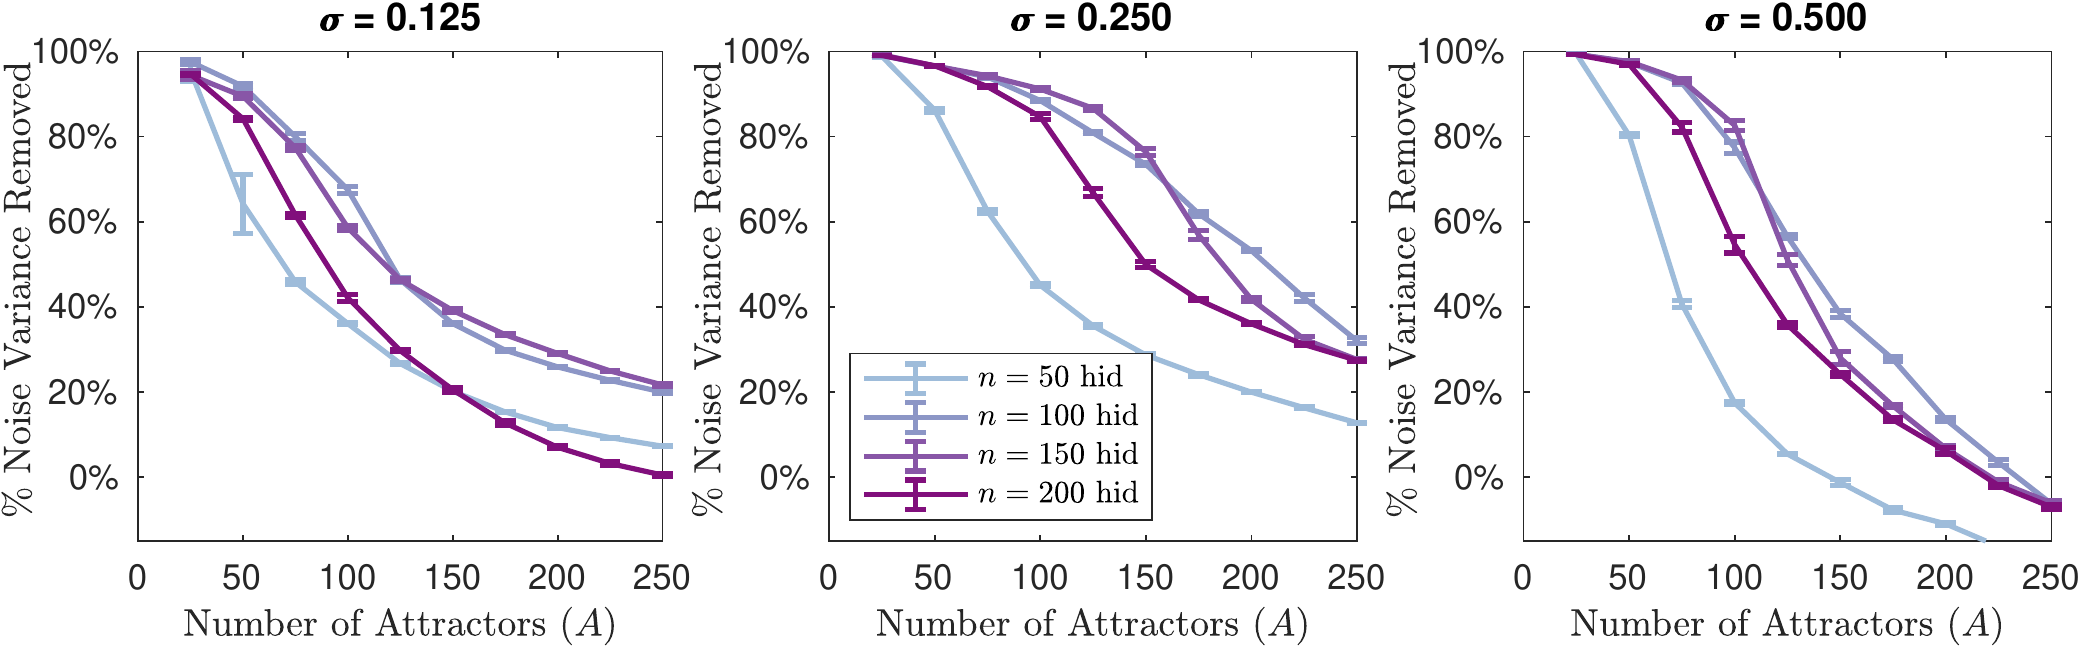}
   \end{center}
   \caption{Percentage noise variance suppression by an attractor net trained 
   on 3 noise levels ($\sigma$). In each graph, the number of hidden units in the attractor net ($n$) and number of attractors to be learned ($A$) is varied.  In all cases, inputs are 50-dimensional and evaluation is based on a fixed $\sigma=0.250$. Ten replications are run of each condition; error bars indicate $\pm1$ SEM.}
   \label{fig:attractor_alone}
\end{figure*}

We trained attractor networks varying the number of target attractor states, $A \in [25, 250]$, the noise corruption, $\sigma\in \{0.125, 0.250, 0.500\}$, and the number of units in the attractor net, $n\in [25, 250]$. In all simulations, the input and output dimensionality is fixed at $m=50$, $\kappa=50$ training inputs and $\kappa=50$ testing inputs were generated for each of the $A$ attractors. The network is run to convergence. Due to the possibility of a limit cycle of 2 steps, we used the convergence criterion $||\bm{y}_{k+2}-\bm{y}_k||_\infty < \delta$, where $\bm{y}_k$ is the output at iteration $k$ of the attractor dynamics. This criterion ensures that no element of the state is changing by more than some small $\delta$. For $\delta=.01$, we found convergence typically in under 5 steps, nearly always under 10.

Figure~\ref{fig:attractor_alone} shows the percentage of noise variance removed by the attractor dynamics on the test set, defined as $100(1-\mathcal{L}_\mathrm{denoise})$. The three panels correspond to different levels of noise in the training set; in all cases, the noise in the test set was fixed at $\sigma=0.250$. The 4 curves each correspond to a different size of the attractor net, $n$. Larger $n$ should have greater capacity for storing attractors, but also should afford more opportunity to overfit the training set. For all noise levels, the smallest ($n=50$) and largest ($n=200$)  nets have lower storage capacity than the intermediate ($n=100,150$) nets, as reflected by a more precipitous drop in noise suppression as $A$, the number of attractors to be stored, increases.
One take-away from this result is that roughly we should choose $n\approx 2m$, that is, the hidden attractor space should be about twice as large as the input/output space. This result does not appear to depend on the number of attractors stored, but it may well depend on the volume of training data. Another take-away from this simulation is that the noise level in training should match that in testing: training with less ($\sigma=0.125)$ and more ($\sigma=0.500)$ noise than in testing ($\sigma=0.250$) resulted in poorer noise suppression. Based on this simulation, the optimal parameters, $\sigma=0.250$ and $n=100$, should yield a capacity for the network that is roughly $2n$, as indicated by the performance drop that accelerates for $A>100$.

\subsection{Attractor net initialization}
We initialize the attractor net with all attractor weights being drawn from a normal distribution with mean zero and standard deviation .01. Additionally, we add 1.0 to the on-diagonal weights of $\bm{W}^\textsc{in}$ and $\bm{W}^\textsc{out}$, i.e., $W^\textsc{in}_{ii}=1+\epsilon$ and $W^\textsc{out}_{ii}=1+\epsilon$~~ for $i \le \min(m,n)$, where $\epsilon \sim \mathcal{N}(0,.01)$ and $m$ is the number of units in the input to the attractor net and $n$ is the number of internal (hidden) units in the attractor net.

\section{Experimental details}

In all experiments, we chose a fixed initial learning rate with the ADAM optimizer. We used the same learning rate for $\mathcal{L}_\mathrm{denoise}$ and $\mathcal{L}_\mathrm{task}$. For all tasks, $\mathcal{L}_\mathrm{task}$ is mean squared error. For the synthetic simulations (parity, majority, Reber, and symmetry), we trained for a fixed upper bound on the number of epochs but stopped training if the training set performance reached asymptote. (There was no noise in any of these data sets, and thus performance below 100\% is indicative that the network had not fully learned the task. Continuing to train after 100\% accuracy had been attained on the training set tended to lead to overfitting, so we stopped training at that point. In all simulations, for testing we use the weights that achieve the highest accuracy on the training set (not the lowest loss).

\subsection{Parity}
We use mean squared error for $\mathcal{L}_{task}$ in Parity, Majority, Reber, and Symmetry.
In Parity, the learning rate is .008 for $\mathcal{L}_\mathrm{task}$ and $\mathcal{L}_\mathrm{denoise}$. Because the data set is noise free, training continues until classification accuracy on the training set is 100\% or until 5000 epochs are reached. Training is in complete batches.  Hidden units are tanh, and the data set has a balance on expectation of positive and negative examples. Our entropy calculation is based on discretizing each hidden unit to 8 equal-sized intervals in $[-1,+1]$ and casting the 10-dimensional hidden state into one of $10^8$ bins. For this and only this simulation, the attractor weights were trained only on the attractor loss. In all following simulations, the attractor weights are trained on both losses (as described in the main text). This change was due to an evolution in our approach, not because we tried both and attractor-loss-only training was necessary.

\begin{figure}[b!]%[100]%[bt]
   \begin{center}
   \includegraphics[width=3.25in]{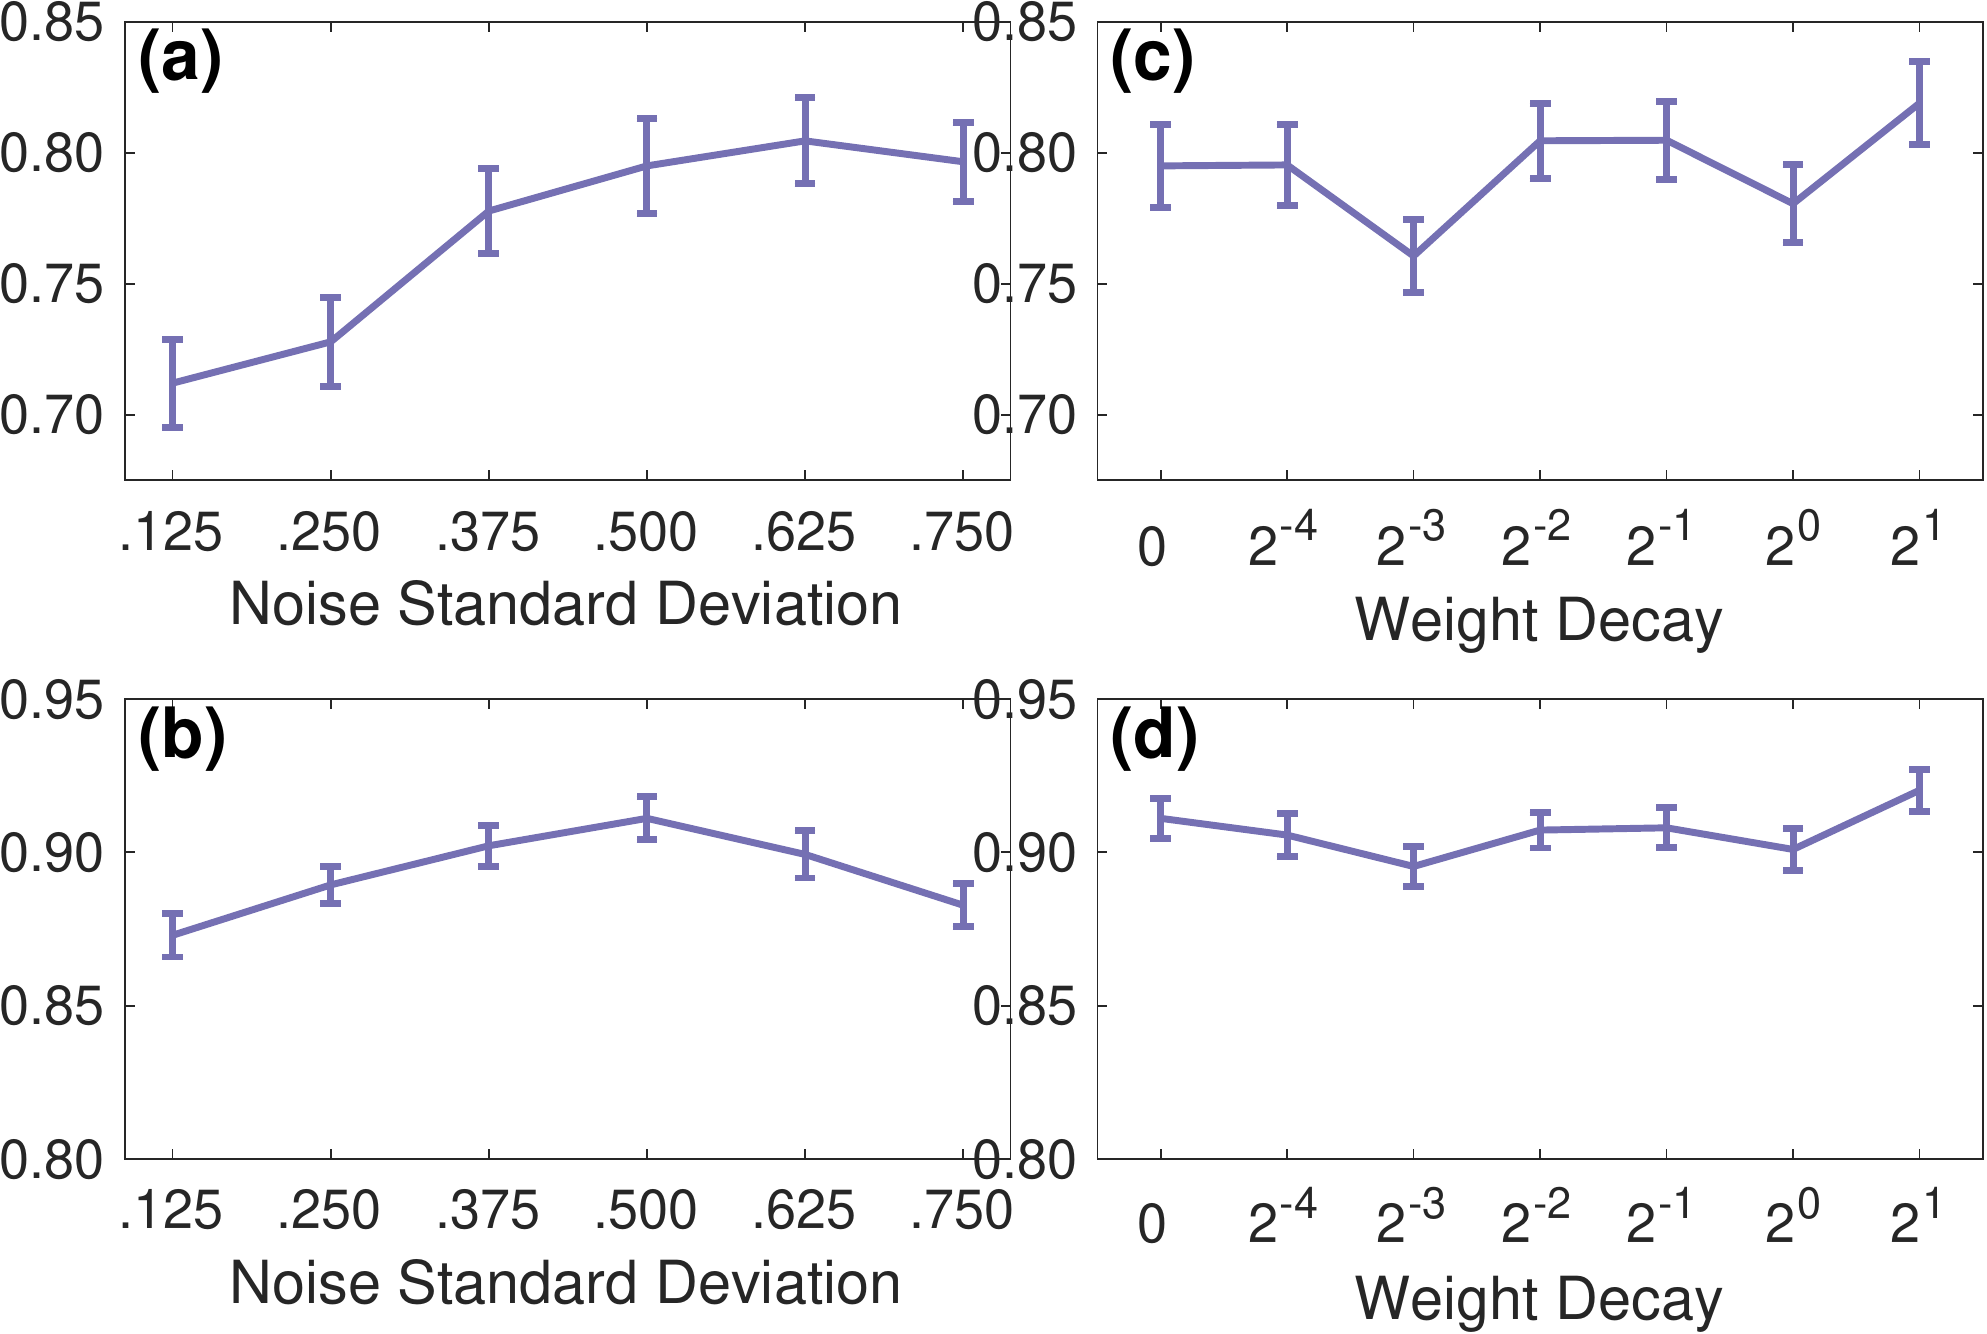}
   \end{center}
   \caption{Parity simulations. Top row shows generalization performance on novel binary sequences; bottom row shows performance on trained sequences with additive noise. Unless otherwise noted, the simulations of the SDRNN use $\sigma=0.5$, 15 attractor iterations, and $L_2$ regularization (a.k.a. weight decay) 0.0. Error bars indicate $\pm1$ SEM, based on a correction for confidence intervals with matched comparisons \citep{MassonLoftus2003}.}
   \label{fig:parity}
\end{figure}

Figure~\ref{fig:parity}a,b show the effect of varying $\sigma$ in training attractors. If $\sigma$ is too small, the attractor net will do little to alter the state, and the model will behave as an ordinary RNN. If $\sigma$ is too large, many states will be collapsed together and performance will suffer. An intermediate $\sigma$ thus must be best,  although what is `just right' should turn out to be domain dependent.
%%% REMOVED FOR SPACE
We explored one additional manipulation that had no systematic effect on performance. We hypothesized that because the attractor-net targets change over the course of learning, it might facilitate training to introduce weight decay in order to forget the attractors learned early in training. We introduced an $L_2$ regularizer using the ridge loss, $\mathcal{L}_\mathrm{ridge} = \lambda || \bm{W} ||_2^2$, where $\bm{W}$ is the symmetric attractor weight matrix in Equation~\ref{eq:att_dyn} and $\lambda$ is a weight decay strength. As Figures~\ref{fig:parity}c,d indicate, weight decay has no systematic effect, and thus, all subsequent experiments use a ridge loss $\lambda=0$. 

\subsection{Majority}
The networks are trained for 2500 epochs or until perfect classification accuracy is achieved on the training set. The attractor net is run for 5 steps. Ten hidden units are used and $\sigma = 0.25$. On expectation there is a balance between the number of positive and negative examples in both the training and test sets.

\subsection{Reber}
The networks are trained for 2500 or until perfect classification accuracy is achieved on the training set. We filtered out strings of length greater than 20, and we left padded strings with shorter lengths with the begin symbol, \textsc{b}. The training and test sets had an equal number of positive and negative examples. The architecture included $m=20$ hidden units and $n=40$ attractor units, and the attractor net is run for 5 steps.
Without exploring alternatives, we decided to postpone the introduction of $\mathcal{L}_\mathrm{denoise}$ until 100 epochs had passed.

\subsection{Symmetry}
The networks are trained for 2500 or until perfect classification accuracy is achieved on the training set. A learning rate of .002 was used for both losses for $f=10$ and .003 for both losses for $f=1$. The attractor net was run for 5 iterations.
